# Supplementary material for: Laser-Induced Magnetic Nanostructures with Tunable Topological Properties
Source: arXiv:1304.1754 source file (2013-04-05)
Supplement: Supplementary file 1 [file Supp._Inf.pdf]

## Laser-Induced Magnetic Nanostructures with Tunable Topological Properties

M. Finazzi,[1] M. Savoini,[1,2] A. R. Khorsand,[2] A. Tsukamoto,[3] A. Itoh,[3] L. Duò,[1] A. Kirilyuk,[2] Th.Rasing,[2] and M. Ezawa.[4]

[1] *Dipartimento di Fisica, Politecnico di Milano, Piazza Leonardo da Vinci 32, 20133 Milano, Italy*
[2] *Radboud University Nijmegen, Institute for Molecules and Materials, Heyendaalseweg 135, 6525 AJ Nijmegen, The Netherlands*
[3] *College of Science and Technology, Nihon University, 7-24-1 Funabashi, Chiba, Japan*
[4] *Department of Applied Physics, University of Tokyo, Hongo 7-3-1, 113-8656, Japan*

### Supplemental Material

*Model Hamiltonian*

We use a classical spin field of unit length, $\mathbf{n} = (n_x, n_y, n_z)$ to describe the spin texture, assuming that its characteristic length scale is much larger than the lattice constant $a$. The Hamiltonian consists of the sum of the anisotropic nonlinear sigma term $H_J = H_X + H_A$ (with $H_X$ and $H_A$ being the exchange interaction and the uniaxial single-ion anisotropy, respectively), the dipole-dipole interaction (DDI) term $H_D$ and the Zeeman term $H_Z$, whose continuous versions read

$$H_X = \frac{1}{2}\Gamma\int(\partial_k\mathbf{n})(\partial_k\mathbf{n})\,d^2r\ , \qquad \text{(S1a)}$$

$$H_A = \frac{1}{2\xi^2}\Gamma\int\left(1-n_z^2\right)d^2r, \qquad \text{(S1b)}$$

$$H_D = H_D^{(1)} + H_D^{(2)} = -\frac{\Omega}{4\pi}\int\left\{\frac{1-\mathbf{n}(\mathbf{r})\cdot\mathbf{n}(\mathbf{r}')}{|\mathbf{r}-\mathbf{r}'|^3} + \frac{3[\mathbf{n}(\mathbf{r})\cdot(\mathbf{r}-\mathbf{r}')][\mathbf{n}(\mathbf{r}')\cdot(\mathbf{r}-\mathbf{r}')]}{|\mathbf{r}-\mathbf{r}'|^5}\right\}d^2r\,d^2r'\ , \qquad \text{(S1c)}$$

$$H_Z = \Delta_Z\int\frac{1-n_z}{a^2}\,d^2r, \qquad \text{(S1d)}$$

where $\Gamma$ is the exchange constant, $\xi$ is the single-ion uniaxial anisotropy, $\Omega$ is the DDI strength, and $\Delta_Z$ is the Zeeman energy. The term $H_D$ represents the DDI between two spins at $\mathbf{r}$ and $\mathbf{r}'$. The ground-state solutions of $H_J$ are $\mathbf{n} = (0, 0, \pm 1)$, i.e. a spin-polarized homogeneous state. Here, we take $\mathbf{n} = (0, 0, 1)$ as the ground state. Note that we have subtracted the ground-state contributions from eqs. S1a-d. In fact, we need to evaluate the net energy of the soliton in order to verify its stability, while the ground-state energy diverges in an infinitely extended two-dimensional magnetic film, and has no physical meaning by itself.

*Solitons*

In principle, soliton solutions are determined by solving the integro-differential equation that follows from the Hamiltonian $H = H_X + H_A + H_D + H_Z$. Since it is not possible to solve it analytically, we just consider a set of reasonable trial functions and determine the one that minimizes the total energy. In particular, we restrict our analysis to spin textures characterized by cylindrical symmetry, which have the following general form:

$$n_x = \mp\sqrt{1-\sigma^2(r)}\cos\varphi(\theta)\,,\qquad n_y = \mp\sqrt{1-\sigma^2(r)}\sin\varphi(\theta)\,,\qquad n_z = \sigma(r), \qquad \text{(S2)}$$

where $\theta$ is the azimuthal angle. The single-valueness of the wave function requires $\varphi(\theta + 2\pi) = \varphi(\theta) + 2n\pi$ with $n$ integer, and $\sigma(0)$ equal to either +1 or –1 in the origin ($r = 0$). For this class of functions, the Pontryagin number is calculated to be $Q_{Sky} = \pm n\,[\sigma(\infty) - \sigma(0)]/2$, which can be equal to either ±1 or 0.

There are two types of interactions in the Hamiltonian: the long-range DDI and the short-range exchange, anisotropy and Zeeman interactions. The short-range interactions are not only responsible for the spin wave spectrum to have a gap, but also the soliton radial function $\sigma(r)$ to approach the ground-state value $\sigma(\infty) = 1$ exponentially fast outside the core. The soliton energy is almost insensitive to the details of the asymptotic behavior outside the core. For this reason we consider a trial function with the following Gaussian form

$$\sigma(r) = 1 - f(r)\,e^{-(r/R)^2}\,, \qquad \text{(S3)}$$

with $R$ being a free parameter defining the size of the soliton and $f(r)$ is a polynomial satisfying the boundary condition $f(0) = 2$ or $f(0) = 0$.

*Skyrmions*

Skyrmions are obtained when $Q_{\mathrm{Sky}} = \pm 1$, which is obtained when $n = 1$ and $f(0) = 2$. The simplest spin texture satisfying the first condition is given by $\varphi(\theta) = \theta + \theta_0$. We consider a class of trial functions such that $f(r) = 2 + \alpha(r/R)^2$. The condition $+1 \geq \sigma(r) \geq -1$ implies that $2 \geq \alpha \geq 0$. The minimum energy is reached at the boundary point $\alpha = 0$, which yields the Skyrmion texture described by eq. 3 in the main text. Substituting this trial function with $R = R_1$ into the Hamiltonian, we estimate the energy contributions as

$$E_{\mathrm{X}}^{0} = \pi\Gamma\left(\frac{\pi^2}{3} + \ln 4\right), \tag{S4a}$$

$$E_{\mathrm{A}}^{0} = \pi\Gamma\frac{R_1^2}{\xi^2}, \tag{S4b}$$

$$E_{\mathrm{D}}^{0} = -\frac{2}{d_f}R_1^2\Omega - \sqrt{2\pi}\left(\sinh^{-1}1 + \sqrt{2} - 1\right)R_1\,\Omega + \sqrt{2}\,d_f\Omega, \tag{S4c}$$

$$E_{\mathrm{Z}}^{0} = 2\pi\frac{R_1^2}{a^2}\Delta_z, \tag{S4d}$$

where we have only kept the first term $H_{\mathrm{D}}^{(1)}$ in the DDI energy (eq. S1c), since it is the dominant one. By minimizing the total energy $E_{\mathrm{X}}^{0} + E_{\mathrm{A}}^{0} + E_{\mathrm{D}}^{0} + E_{\mathrm{Z}}^{0}$ with respect to the free parameter $R_1$, the Skyrmion size $R_1$ is given by eq. 4 in the text.

*Skyrmionium*

We may also consider a class of trial functions possessing a total Skyrmion number $Q_{\mathrm{Sky}} = 0$. Although these structures are not protected by topological stability, according to the Derrick-Hobart theorem such solitons can nevertheless be dynamically stable. A nontopological spin texture is obtained when $f(0) = 0$. We consider a class of functions such that $f(r) = \alpha(r/R)^2$. The condition $1 \geq \sigma(r) \geq -1$ implies that $2e \geq \alpha \geq 0$. There are energy minima at the boundary points: $\alpha = 0$ yields the ground state, while $\alpha = 2e$ yields the Skyrmionium spin texture described by eq. 5 in the main text. Substituting this trial function with $R = R_0$ into the Hamiltonian, we are able to analytically estimate the total energy (again, we only consider the first term $H_{\mathrm{D}}^{(1)}$ in the DDI energy):

$$E_{\mathrm{X}}^{0} = \pi\Gamma\left(\frac{e(4-e)}{2} + 13.6\right), \tag{S5a}$$

$$E_{\mathrm{A}}^{0} = \pi\Gamma\frac{e(4-e)}{2}\frac{R_0^2}{\xi^2}, \tag{S5b}$$

$$E_{\mathrm{D}}^{0} = -\frac{e(4-e)}{d_f}R_0^2\Omega - \sqrt{\frac{\pi}{2}}\left(2 + \ln 3\right)e\,R_0\,\Omega, \tag{S5c}$$

$$E_{\mathrm{Z}}^{0} = 2\pi\frac{R_0^2}{a^2}\Delta_z, \tag{S5d}$$

where we have used the following relation:

$$\int_0^\infty \frac{\left[\partial_r\sigma(r)\right]^2}{1-\sigma(r)^2}r\,dr = 13.6. \tag{S6}$$

By minimizing the total energy $E_{\mathrm{X}}^{0} + E_{\mathrm{A}}^{0} + E_{\mathrm{D}}^{0} + E_{\mathrm{Z}}^{0}$, the Skyrmionium size $R_0$ is given by eq. 6 in the main text. We have also checked that the relation $E_{\mathrm{A}}^{0} + E_{\mathrm{Z}}^{0} = E_{\mathrm{D}}^{0}$ holds for the above solution.
